# Supplementary material for: Learning Priors for Adversarial Autoencoders
Source: arXiv:1909.04443 source file (2019-09-10)
Supplement: Supplementary file 1 [file appendix.tex]

\appendices
\section{Implementation details}
\label{sec:appendix_model_arch}
Table \ref{table:enc_dec_mnist}, Table \ref{table:cg_mnist}, and Table \ref{table:disc} presents the implementation details of each components in our model. Each cell in the tables presents the type of neural networks, the output size, w/o batch normalization, the type of activation function, the size for strides, and the size of padding. Lastly, Fig.~\ref{fig:detailed_arch} presents the detailed architecture of the proposed model.

\begin{table}[tbp]
%\centering
\caption{Implementation details of the encoder and decoder networks}
\label{table:enc_dec_mnist}
\begin{tabular}{l|l}
\hline
Encoder                                         & Decoder                                       \\ \hline
Input 32 x 32 images                			& Input latent code $\in R^{code \: size}$      \\ \hline
3 x 3 conv. 64 RELU stride 2 pad 1              & 4 x 4 upconv. 512 BN. RELU stride 1           \\ \hline
3 x 3 residual blcok 64                         & 4 x 4 up sampling residual block 256 stride 2 \\ \hline
3 x 3 down sampling residual blcok 128 stride 2 & 4 x 4 up sampling residual block 128 stride 2 \\ \hline
3 x 3 down sampling residual blcok 256 stride 2 & 4 x 4 up sampling residual block 64 stride 2  \\ \hline
3 x 3 down sampling residual block 512 stride 2 & 3 x 3 conv. image channels Tanh                           \\ \hline
4 x 4 avg. pooling stride 1                     &                                               \\ \hline
FC. 2 x code size BN. RELU                      &                                               \\ \hline
FC. code size Linear                            &                                               \\ \hline
\end{tabular}
\end{table}

\begin{table}[btp]
\centering
\caption{Implementation details of the code generator networks}
\label{table:cg_mnist}
\begin{tabular}{l|l}
\hline
Code Generator                  	 & Residual block                                \\ \hline
Input noise $\in R^{noise \: size}$  & Input feature map                             \\ \hline
FC. 2 x noise size BN. RELU    		 & 3 x 3 conv. out\_channels RELU stride 2 pad 1 \\ \hline
FC. latent code size BN. Linear      & 3 x 3 conv. out\_channels RELU stride 1 pad 1 \\ \hline
	                                 & skip connection output = input + residual     \\ \hline
                                     & RELU                                              \\ \hline
\end{tabular}
\end{table}

\begin{table}[]
\centering
\caption{Implementation details of the image and code discriminator}
\label{table:disc}
\begin{tabular}{ll}
\hline
Image Discriminator $D$/$Q$                                       & Code Discriminator \\ \hline
Input 32 x 32 images                                       & Input latent code  \\ \hline
4 x 4 conv. 64  LRELU stride 2 pad 1                       & FC 1000 LRELU      \\ \hline
4 x 4 conv. 128 BN LRELU stride 2 pad 1                    & FC 500 LRELU       \\ \hline
4 x 4 conv. 256 BN LRELU stride 2 pad 1                    & FC 200 LRELU       \\ \hline
FC. 1000 LRELU                                             & FC 1 Sigmoid       \\ \hline
FC 1 Sigmoid for $D$                                         &                    \\ \hline
FC 10 Softmax for $Q$                                        &                    \\ \hline
\end{tabular}
\end{table}
